# Supplementary material for: Yielding and microstructure in a 2D jammed material under shear deformation
Source: arXiv:1304.2253 ancillary file (2013-05-28)
Supplement: Supplementary file 1 [file supplemental.pdf]

# Supplementary Material for "Yielding and microstructure in a 2D jammed material under shear deformation"

N.C. Keim and P.E. Arratia

May 28, 2013

## 1 Materials and Methods

### 1.1 Interfacial material

The interfacial material is a bidisperse (equal parts by number) mixture of 4.1 and 5.6 $\mu$m-diameter sulfate latex (polystyrene) particles (Invitrogen; nominal diameters 4 and 6 $\mu$m) adsorbed at the interface between deionized water and decane.[1–3] Area fraction $\phi$ is set by the number of particles dispersed into the experimental cell, a 6 cm-diameter glass dish; positive osmotic surface pressure keeps $\phi$ uniform. Particles are rinsed 4 times in deionized water, then resuspended in a water-ethanol mixture (50% by volume) to ensure dispersion at the interface. To remove polar contaminants, decane (Acros Organics, "99+%") is treated with aluminum oxide powder, which is then removed by filtration. All other components are cleaned by repeated sonication and rinsing in deionized water and ethanol.

### 1.2 Interfacial stress rheometer

A static Helmholtz field keeps the needle centered in the channel, while another electromagnet moves the needle back and forth, uniformly shearing the interface in the channel. The equation of motion[4] for the needle position $x$ is

$$m\ddot{x} = AI_{\text{drive}} - kx - d\dot{x} - F_s \tag{1}$$

where $m$ is the needle mass, $AI_{\text{drive}}$ is the force from the computer-controlled driving current, $k$ is the spring constant for the central potential of the Helmholtz field, $d$ represents drag from the bulk fluid, and $F_s$ is due to any material adsorbed at the surface. If $m$ is known, the values of $a$, $k$, and $d$ may be determined by applying a sinusoidal $I_{\text{drive}}$ on a clean interface at a range of frequencies, allowing computation of $F_s(t)$ from $x(t)$, and so permitting measurement of the oscillatory rheology of a material. We obtain $x(t)$ by tracking the first $\sim 5$ layers of particles at the needle,[5] which we validate visually by observing the

motion of irregularities on the surface of the needle itself. The material response is modeled as $\sigma(t) = (G' + iG'')\gamma_0 e^{i\omega t}$, where $\sigma$ is the stress applied to the material, $\gamma_0$ is the strain amplitude, $\omega$ is the driving frequency, and $G'$ and $G''$ are the elastic and loss moduli.

Decoupling of the rheology of the surface from that of the bulk fluids above and below it is characterized by the Boussinesq number $Bq = |\eta_i^*|/\eta_b a$, the dimensionless ratio of interfacial and bulk stresses, where $\eta_i^*$ is the complex interfacial viscosity, $\eta_b$ is the bulk fluid viscosity, and $a$ is the diameter of the needle.[4,6] Here $Bq \sim 100$, so that to a good approximation we measure only the interfacial rheology, and stress is applied to the material only at its boundaries.

## 1.3 Particle tracking and T1 events

The material is imaged during shear with a long-distance microscope (K2/SC with CF-3 objective and CF amplifier, Infinity Photo-Optical) and high-speed camera (Flare 4M180, IOIndustries), imaging with a resolution of $\sim 1.1$ $\mu$m/pixel at up to 150 frames/s. Particles are illuminated with diffuse light from below. With few exceptions, all particles are tracked[5] for the entirety of each movie (thousands of frames).

### 1.3.1 Boundary conditions

Because we can see clearly a single adsorbed layer of particles on the needle, we know that we can track nearly all of the particles at this boundary, and that slippage is minimal. However, some particles near the wall are hidden, due to imperfect alignment of the wall with the microscope line-of-sight. The actual position of the wall is inferred by fitting a straight line to a such a displacement profile for small $\gamma_0$, when deformation was most affine; this suggests that $\sim 12$ layers of particles are hidden. This single inferred position was then used to correct all of the profiles in Fig. 1 of this supplementary information. The hidden particles do not form a slip region: the last visible layer before the wall does not exhibit net creep, and its displacements stay in proportion to the global $\gamma_0$, deviating only at the largest $\gamma_0 = 0.07$ (supplementary Fig. 1). Furthermore, an examination of the spatial distribution of rearrangement activity in Fig. 4 of the paper suggests that there is no undue concentration of activity in this hidden region which would significantly change our results.

### 1.3.2 Detection of T1 events

To measure change to microstructure, nearest-neighbor relationships among particles are computed by Delaunay triangulation.[7] While T1 events are more fundamental to the dynamics of 2D foams,[8] here nearest neighbors also dominate, with the repulsion force scaling as $\sim r^{-4}$.[2] We remove the least significant events by requiring both that the topology be altered and that

$$-\frac{(r_{12}^0 - r_{12}^1)(r_{34}^0 - r_{34}^1)}{(r_{12}^0 + r_{12}^1)(r_{34}^0 + r_{34}^1)} \geq 5 \times 10^{-3}. \quad (2)$$

where $r_{12}$ and $r_{34}$ are the separations of the particle pairs in the T1 event (see Fig. 1 of main text) and the superscripts 0 and 1 denote the times at which particle positions are compared. Lowering this threshold to $10^{-4}$ effectively adds a noise floor of $\sim 10$ events per cycle to all movies in Fig. 2 of the text (even at $\gamma_0 = 1.1 \times 10^{-3}$), but otherwise leaves the qualitative results unchanged. Our specific method undercounts T1s when a particle is involved in many successive events over a cycle, but is appropriate for the experiments presented here, in which rearrangements become rare.

#### 1.3.3 Timescale and discrete nature of T1 events

We may estimate the microscopic relaxation timescale $\tau_r$ for the particles in a T1 rearrangement to come approximately to rest in their new topology. We model the interparticle repulsion that drives rearrangements as a harmonic spring with constant $\mathcal{O}(G')$, where $G'$ is the bulk elastic modulus measured at small $\gamma_0$, when deformation is maximally affine and elastic, and involves only small motions within each interparticle potential. Balancing this repulsion against hydrodynamic drag gives a timescale of $\tau_r = 6\pi\eta R/G' \sim 0.2$ s, where $\eta$ is solvent viscosity and $R$ is particle radius. This comports with a timescale of $\sim 0.5$ s found by visual examination of video. Since $\tau_r \ll f^{-1}$ and $\tau_r \ll \dot{\gamma}_0^{-1}$, the rearrangement timescale is consistent with our modeling of changes to microstructure as discrete events which alter an otherwise quasistatic material.

## 2 Deformation profiles

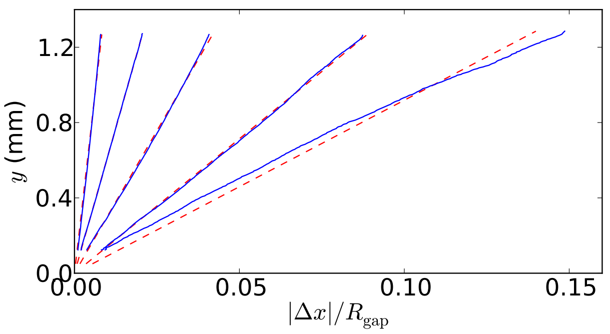


Figure 1: Deformation profiles in the steady state reflect nearly-uniform shear. Net displacement $\Delta x$ of each particle over a half-cycle is shown scaled by the needle-wall distance $R_{\rm gap}$, as a function of distance $y$ of that particle from the wall, averaging over all $x$. Profiles are plotted for $\gamma_0 = 0.004$, 0.01, 0.02, 0.04, and 0.07. Displacements are measured from the last recorded minimum in $\gamma$, backwards to the maximum in $\gamma$ just before it. The red dashed line with each blue curve represents a best-fit line, to guide the eye.

# 3 Creep during oscillatory shear

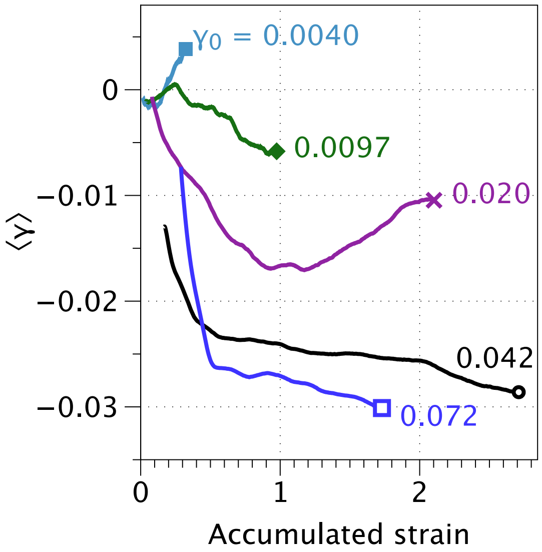


Figure 2: Creep during oscillatory shear shown as evolution of mean strain, computed from needle position as a moving average with a window of length 1 cycle, corresponding to the experiments in Fig. 3a of the paper. The residual bulk stress $\sigma_{\mathrm{DC}}$ from preparation points in the direction of negative $\gamma$. Evolution of $\langle\gamma\rangle$ is much less monotonic and reproducible than the rate of particle rearrangements, suggesting that below yielding, $\sigma_{\mathrm{DC}}$ is less significant than unrelaxed internal stresses.

While our principal results concern the nature of the steady state, the transient regime reveals some key features of the experiment. Figure 2 shows that relaxation in microstructure is accompanied by a bulk creep of the material, as measured from the mean position of the needle. This net deformation relaxes some of the residual stress $\sigma_{\mathrm{DC}}$ from the rheometer. However, our creep measurements are irregular and irreproducible, sometimes even going in the opposite of the expected direction. By contrast, the microstructure results in Figs. 2 and 4e of the paper are remarkably consistent among runs. This leads us to conclude that un-annealed internal stresses are the major source of the free energy associated with relaxation, and that their relaxation is best captured by examining rearrangements.

# 4 Yielding transition in $D^2_{\mathrm{min}}$

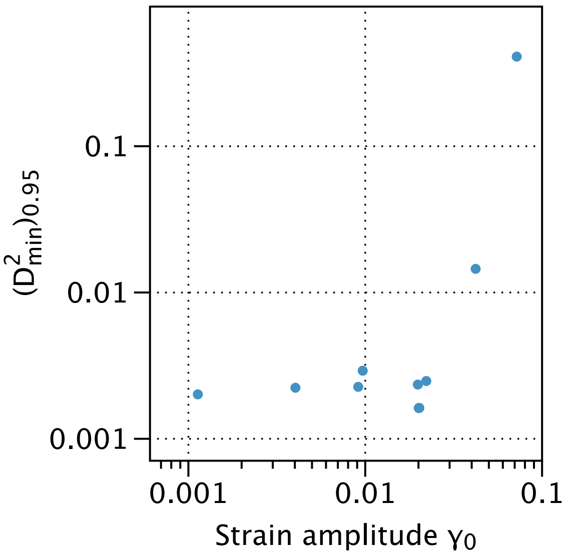


Figure 3: 95th percentile of all particles' $D^2_{\mathrm{min}}$ (shown spatially in Fig. 4 of paper) over final 3 cycles of each movie in Fig. 3 of paper, plotted as a function of strain amplitude. Data demonstrate further the transition to irreversibility that coincides with rheological yielding.

## References


[1] R. Aveyard, J. H. Clint, D. Nees and V. N. Paunov, *Langmuir*, 2000, **16**, 1969–1979.

[2] B. J. Park, J. P. Pantina, E. M. Furst, M. Oettel, S. Reynaert and J. Vermant, *Langmuir*, 2008, **24**, 1686–1694.

[3] K. Masschaele, B. J. Park, E. M. Furst, J. Fransaer and J. Vermant, *Physical Review Letters*, 2010, **105**, 048303.

[4] C. F. Brooks, G. G. Fuller, C. W. Frank and C. R. Robertson, *Langmuir*, 1999, **15**, 2450–2459.

[5] J. C. Crocker and D. G. Grier, *J. Colloid Interf. Sci.*, 1996, **179**, 298–310.

[6] S. Reynaert, C. F. Brooks, P. Moldenaers, J. Vermant and G. G. Fuller, *J. Rheol.*, 2008, **52**, 261–285.

[7] C. B. Barber, D. P. Dobkin and H. Huhdanpaa, *ACM Trans. Math. Softw.*, 1996, **22**, 469–483.

[8] D. Weaire and N. Rivier, *Contemp. Phys.*, 1984, **25**, 59–99.
